# Supplementary material for: BetterV: Controlled Verilog Generation with Discriminative Guidance
Source: arXiv:2402.03375 source file (2024-05-02)
Supplement: Supplementary file 1 [file appendix.tex]

\section{You \emph{can} have an appendix here.}

You can have as much text here as you want. The main body must be at most $8$ pages long.
For the final version, one more page can be added.
If you want, you can use an appendix like this one.
